# Supplementary material for: The intensification of winter mid-latitude storms in the Southern Hemisphere
Source: arXiv:2201.10413 source file (2022-06-02)
Supplement: Supplementary file 1 [file SM_yani.pdf]

# **The intensification of winter mid-latitude storms in the Southern Hemisphere**

Rei Chemke<sup>1</sup> & Yi Ming<sup>2</sup> & Janni Yuval<sup>3</sup>

<sup>1</sup>*Department of Earth and Planetary Sciences, Weizmann Institute of Science, Rehovot, Israel*

<sup>2</sup>*NOAA/Geophysical Fluid Dynamics Laboratory, Princeton, New Jersey, USA*

<sup>3</sup>*Department of Earth, Atmospheric and Planetary Sciences, MIT, Cambridge, Massachusetts, USA*

Table 1: List of the 16 CMIP6 models analyzed in this study and their availability (marked by asterisks).

|    | <b>Model</b>  | <b>EKE</b> | <b>MSE</b> | <b>PI</b> | <b>AMIP6</b> |
|----|---------------|------------|------------|-----------|--------------|
| 1  | ACCESS-CM2    | *          |            |           | *            |
| 2  | ACCESS-ESM1-5 | *          |            |           | *            |
| 3  | CanESM5       | *          | *          | *         | *            |
| 4  | CESM2-WACCM   | *          | *          | *         | *            |
| 5  | CMCC-CM2-SR5  | *          |            | *         | *            |
| 6  | EC-Earth3-Veg | *          |            | *         |              |
| 7  | FGOALS-g3     | *          | *          |           |              |
| 8  | GFDL-CM4      | *          | *          |           | *            |
| 9  | INM-CM4-8     | *          | *          | *         | *            |
| 10 | INM-CM5-0     | *          | *          | *         | *            |
| 11 | IPSL-CM6A-LR  | *          | *          | *         | *            |
| 12 | MPI-ESM1-2-HR | *          | *          | *         | *            |
| 13 | MPI-ESM1-2-LR | *          | *          | *         | *            |
| 14 | MRI-ESM2-0    | *          | *          | *         | *            |
| 15 | NorESM2-LM    | *          | *          |           | *            |
| 16 | NorESM2-MM    | *          | *          |           |              |

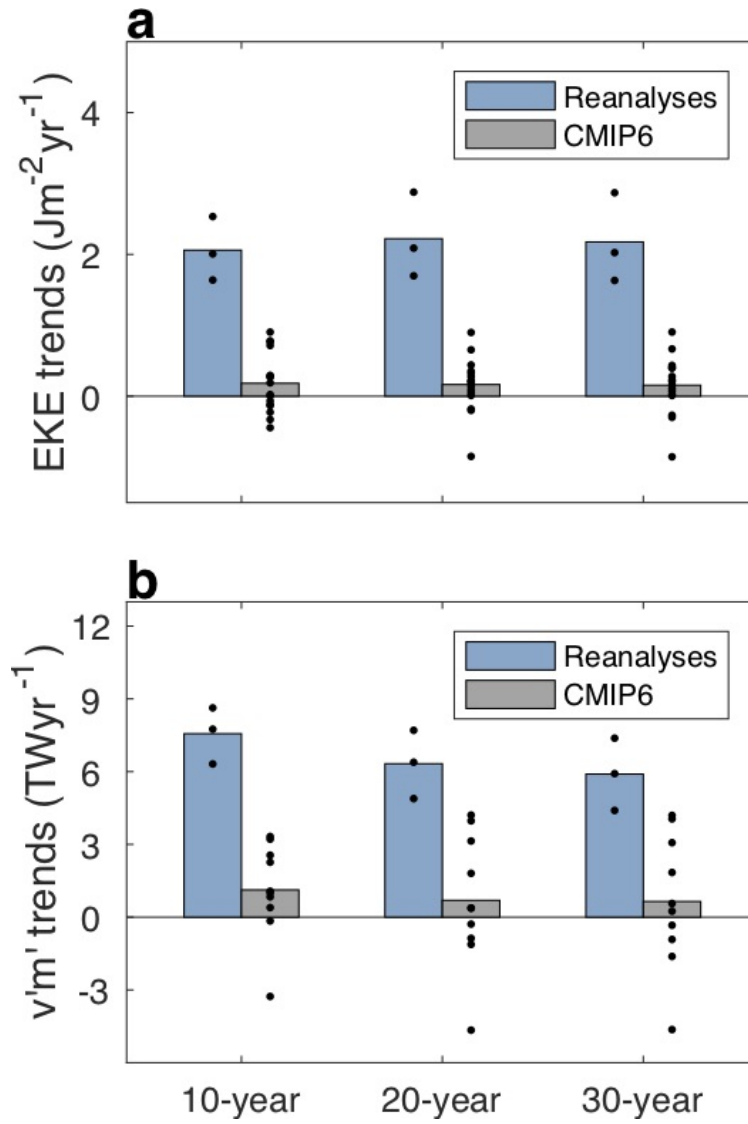

**Fig. S1.** The mean of all 10-year, 20-year and 30-year trends over the 1979-2018 in **a**, eddy kinetic energy and **b**, poleward eddy moist static energy flux in reanalyses mean (blue) and CMIP6 mean (gray). The black circles show the trends from the individual reanalyses/models.

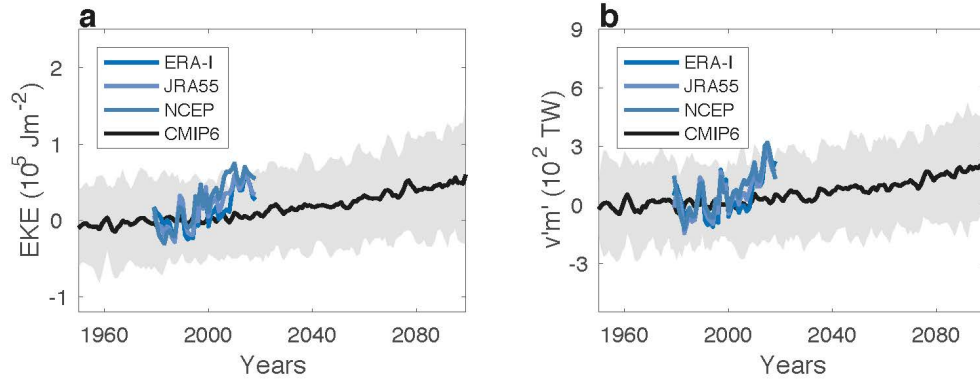

**Fig. S2.** Time evolution of **a**, eddy kinetic energy and **b**, poleward eddy moist static energy flux, relative to the 1980-1999 period, in each reanalyses (blue lines) and CMIP6 mean (black). Shading shows two standard deviations across CMIP6 models. The time evolution is smoothed with a 3-point running mean for plotting purposes.

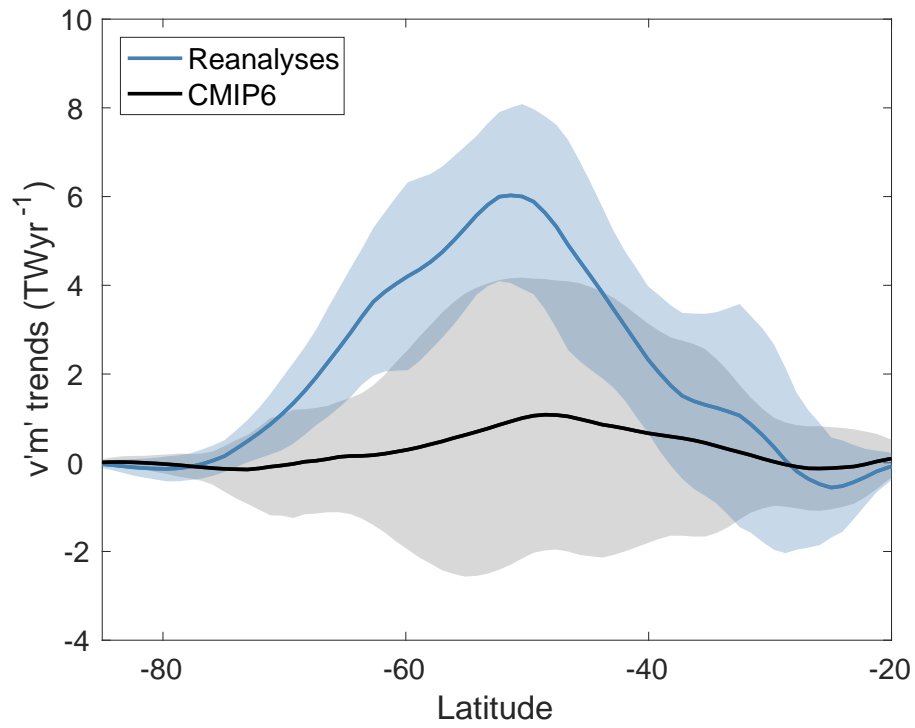

**Fig. S3.** The 1979-2018 trends in poleward eddy moist static energy flux as a function of latitude in reanalyses mean (blue line) and CMIP6 mean (black line). Shadings show two standard deviations across reanalyses/CMIP6 models.

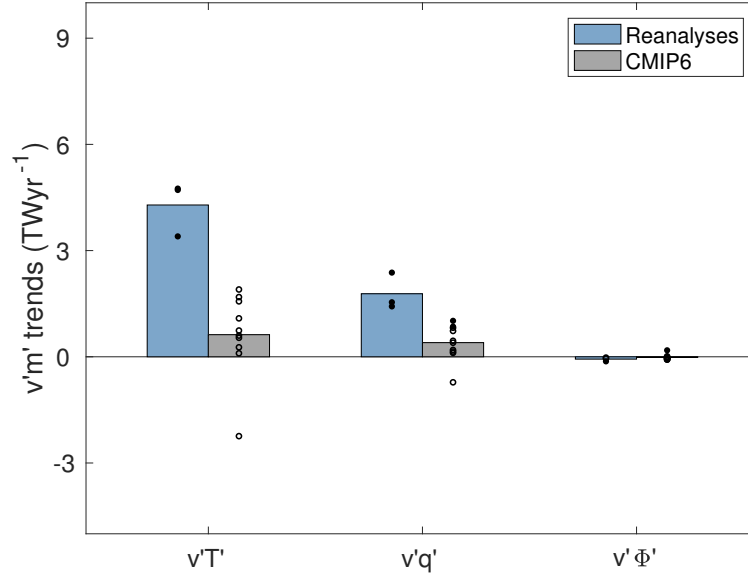

**Fig. S4.** The 1979-2018 trends in poleward eddy moist static energy flux, decomposed to eddy heat flux ( $v'T'$ ), eddy moisture flux ( $v'q'$ ) and eddy geopotential flux ( $v'\Phi'$ ) in reanalyses mean (blue) and CMIP6 mean (gray). The black circles show the trends from the individual reanalyses/models, where filled (open) circles show trends that are (not) statistically significant at the 95% level based on a Student's t-test.

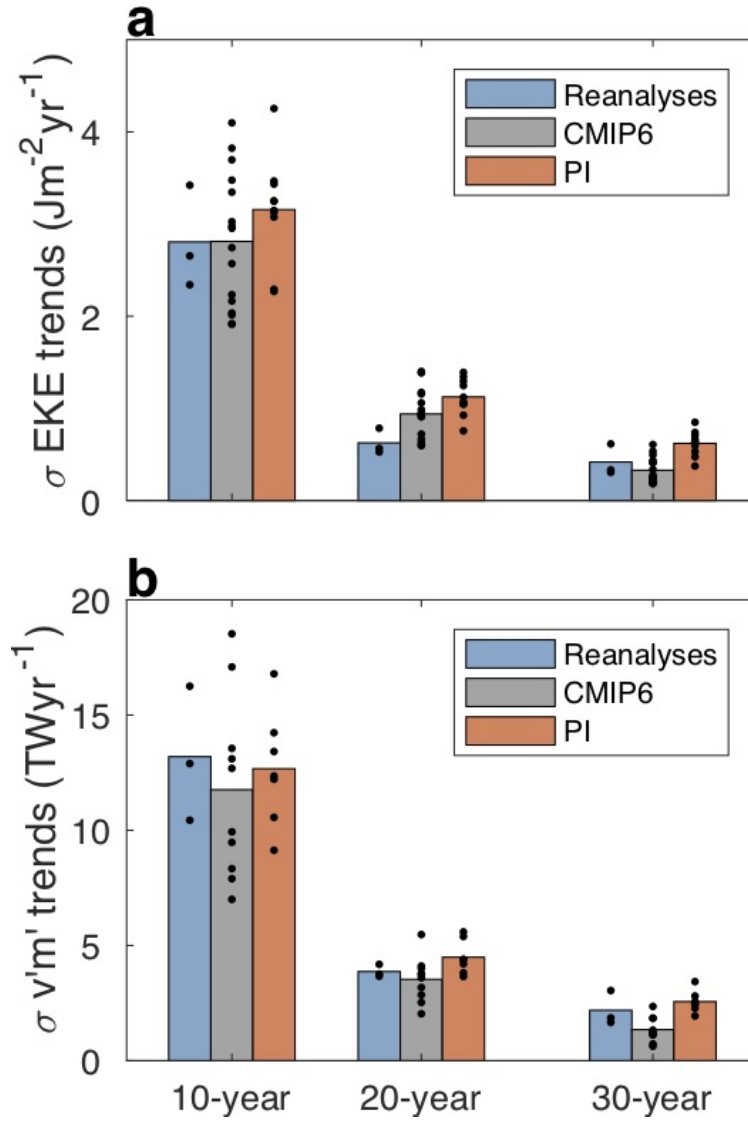

**Fig. S5.** One standard deviation across all 10-year, 20-year and 30-year trends in **a**, eddy kinetic energy and **b**, poleward eddy moist static energy flux in reanalyses mean (blue), CMIP6 mean (gray), and pre-industrial runs (red). The trends in models and reanalyses were calculated over the detrended 1979-2018 period. The black circles show the results from individual reanalyses/models.

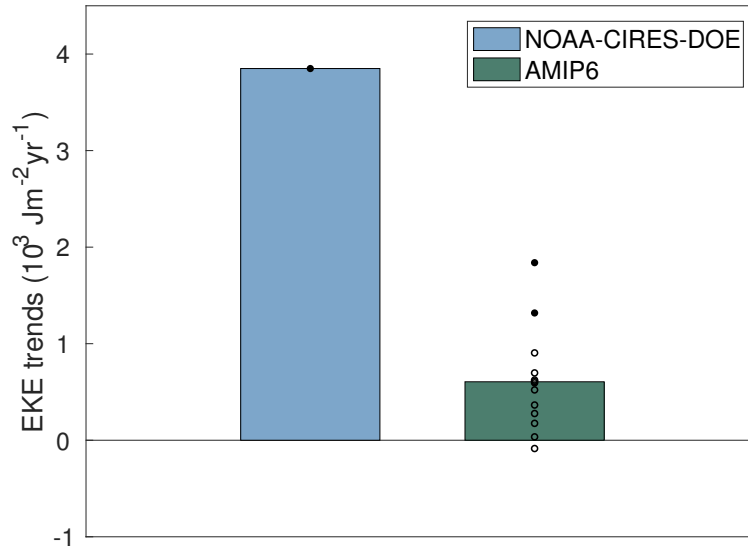

**Fig. S6.** The 1981-2014 trends in eddy kinetic energy in NOAA-CIRES-DOE (blue) and AMIP6 mean (green). The black circles show the trends from the individual models/NOAA-CIRES-DOE, where filled (open) circles show trends that are (not) statistically significant at the 95% level based on a Student's t-test.

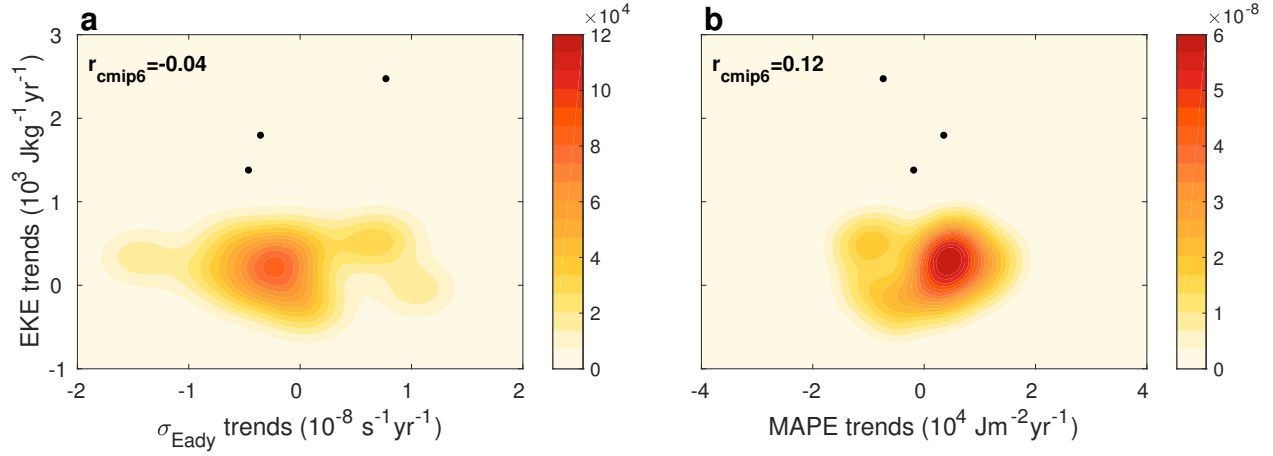

**Fig. S7.** The 1979-2018 eddy kinetic energy trends plotted against the trends in **a**, Eady growth rate and **b**, MAPE. Contours show the two-dimensional probability density function of the trends in CMIP6 models, estimated by fitting a kernel distribution, and the correlation appears in each panel. The black circles show the trends from reanalyses.

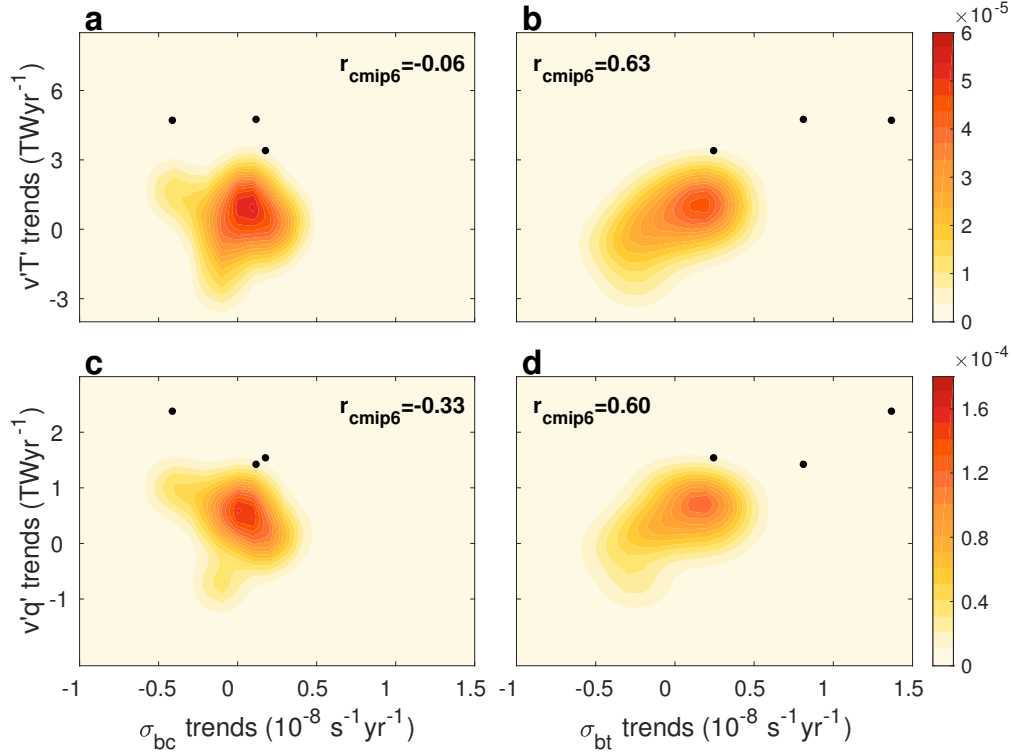

**Fig. S8.** The 1979-2018 trends in eddy heat flux ( $v'T'$ , upper row) and eddy moisture flux ( $v'q'$ , bottom row) plotted against the trends in baroclinic (left column) and barotropic (right column) growth rates of mid-latitude eddies, calculated from a linear normal-mode instability analysis. Contours show the two-dimensional probability density function of the trends in CMIP6 models, estimated by fitting a kernel distribution, and the correlation appears in each panel. The black circles show the trends from reanalyses.

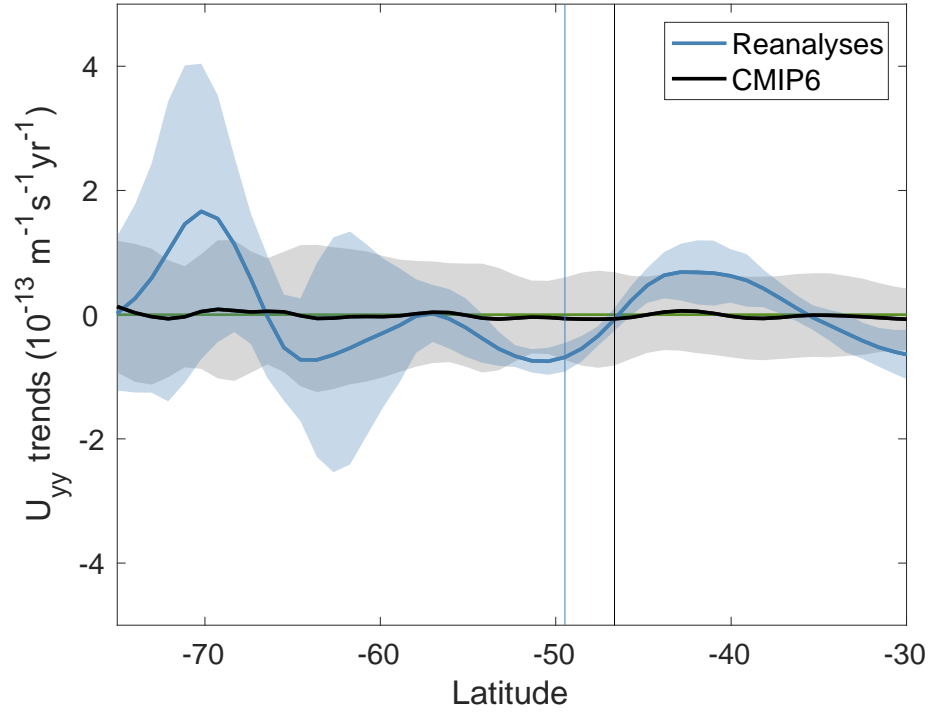

**Fig. S9.** The 1979-2018 trends in the second meridional derivative of the tropospheric (averaged between 850mb – 300mb) mean zonal wind,  $\frac{\partial}{\partial \theta} \frac{1}{r \cos \theta} \frac{\partial \bar{u} \cos \theta}{\partial \theta}$ , in mean reanalyses (blue line) and CMIP6 (black line). Shadings show two standard deviations across reanalyses/CMIP6 models. The vertical lines mark the climatological position of the mean zonal wind's core in reanalyses mean (blue) and CMIP6 mean (black). Green line marks the zero line. The latitudinal structure is smoothed with a 3-point running mean for plotting purposes.

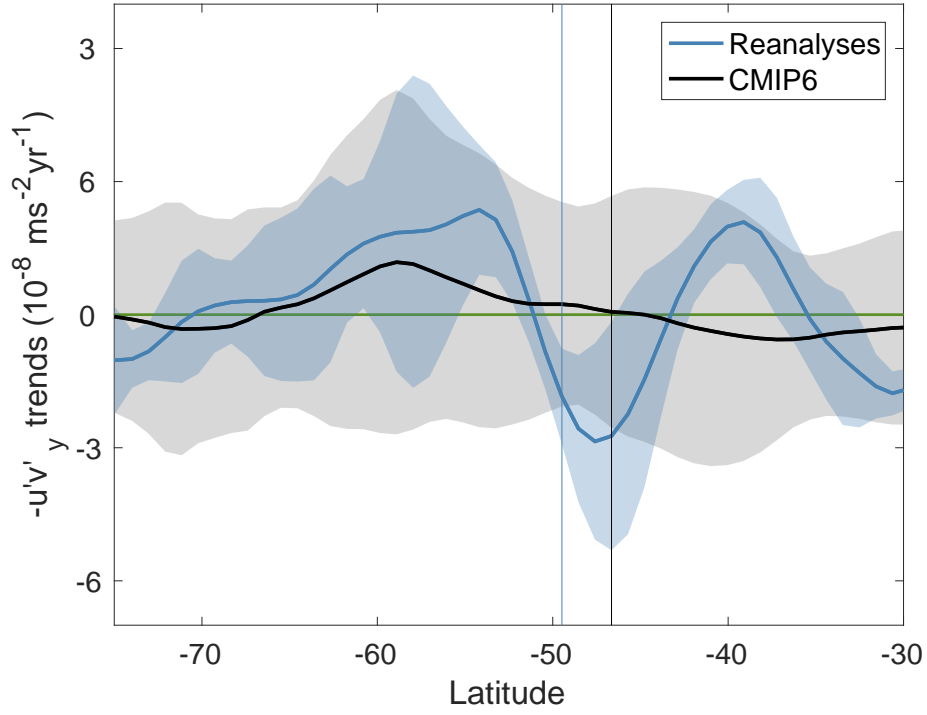

**Fig. S10.** The 1979-2018 trends in vertically averaged eddy momentum flux convergence,  $-\frac{1}{r \cos \theta} \frac{\partial \overline{u'v'} \cos \theta}{\partial \theta}$ , in mean reanalyses (blue line) and CMIP6 (black line). Shadings show two standard deviations across reanalyses/CMIP6 models. The vertical lines mark the climatological position of the mean zonal wind's core in reanalyses mean (blue) and CMIP6 mean (black). Green line marks the zero line. The latitudinal structure is smoothed with a 3-point running mean for plotting purposes.

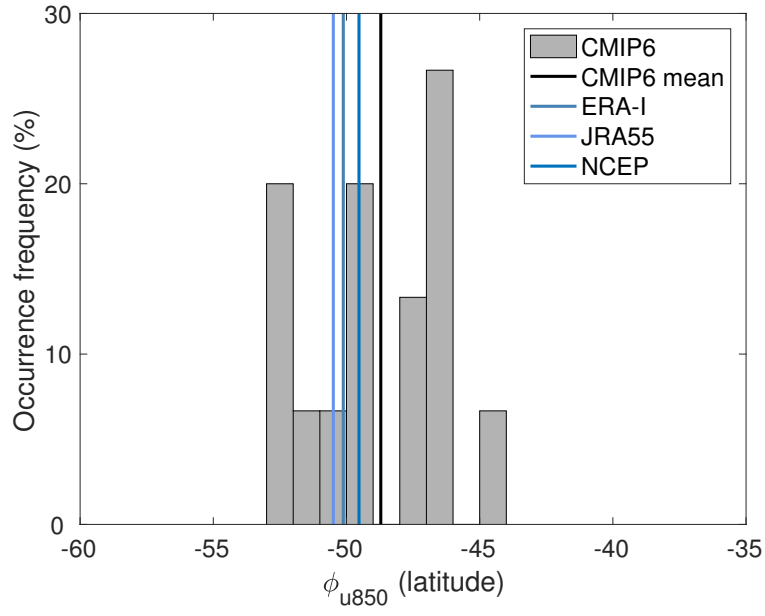

**Fig. S11.** The occurrence frequency of the climatological (averaged over the 1979-2018 period) position of the mean zonal wind's core across CMIP6 models (gray). The vertical blue and black lines show the position of the jet in each reanalysis and in CMIP6 mean, respectively.

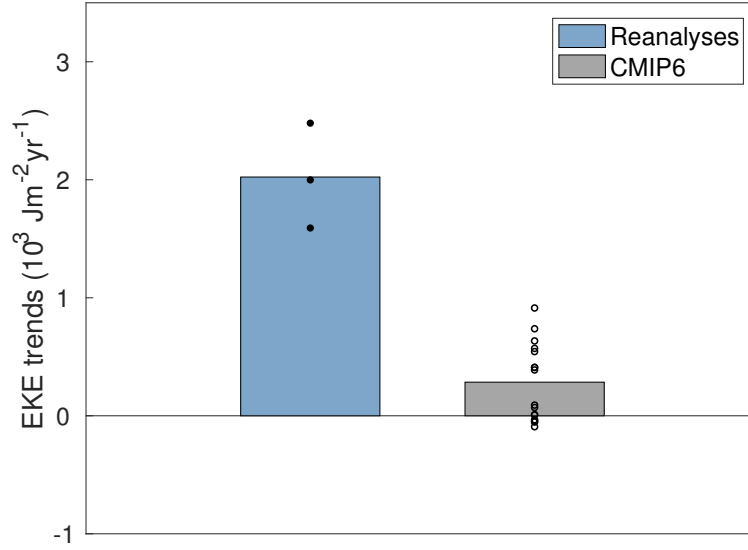

**Fig. S12.** The 1979-2018 trends in eddy kinetic energy in reanalyses mean (blue) and CMIP6 mean (gray). The black circles show the trends from the individual reanalyses/models, where filled (open) circles show trends that are (not) statistically significant at the 95% level based on a Student's t-test. Here the eddy kinetic energy is defined using a bandpass filter of 3-10 days.

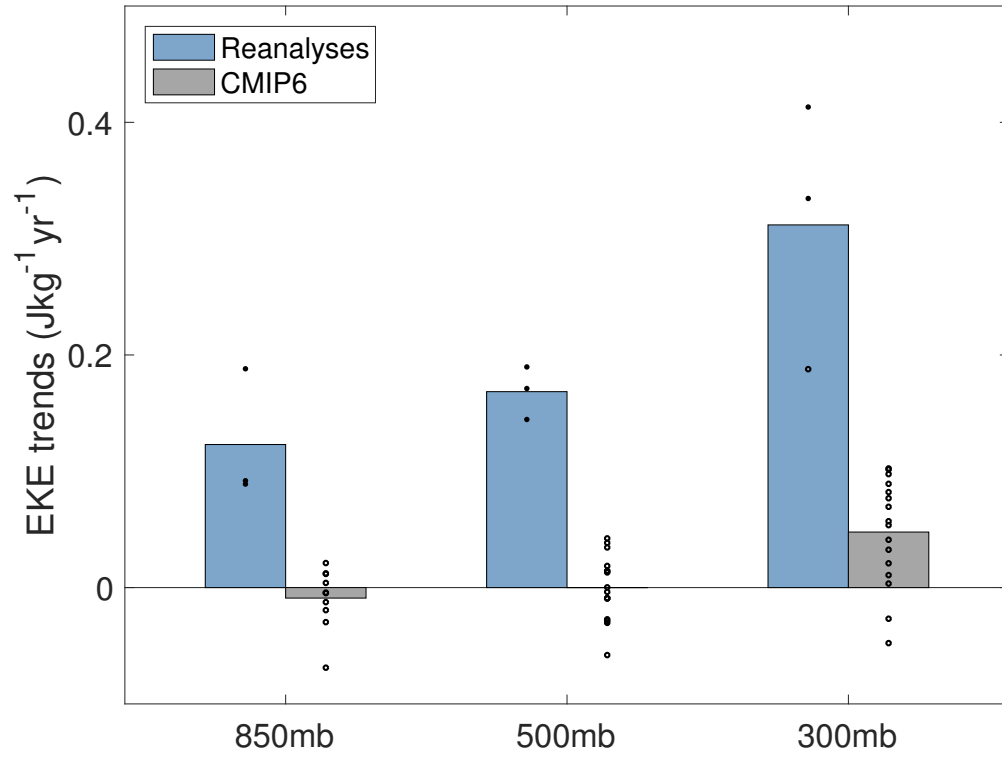

**Fig. S13.** The low-level (850mb), mid-level (500mb) and high-levels (300mb) 1979-2018 trends eddy kinetic energy in reanalyses mean (blue) and CMIP6 mean (gray). The black circles show the trends from the individual reanalyses/models, where filled (open) circles show trends that are (not) statistically significant at the 95% level based on a Student's t-test.

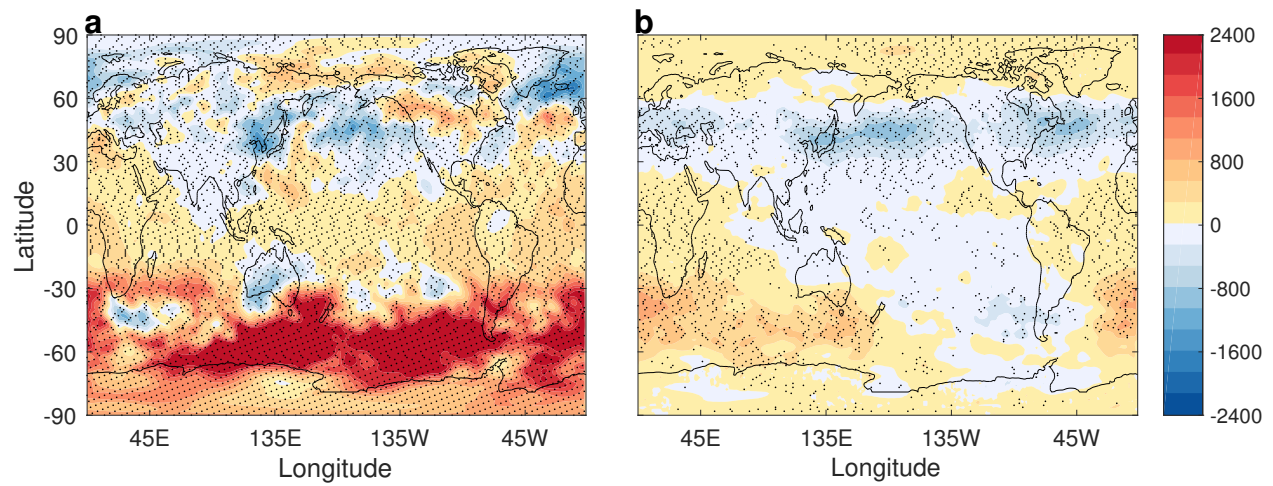

**Fig. S14.** The distribution of the 1979-2018 eddy kinetic energy trends in **a**, reanalyses mean and **b**, CMIP6 mean. The small black dots indicate regions where two thirds of the models/reanalyses agree on the sign.

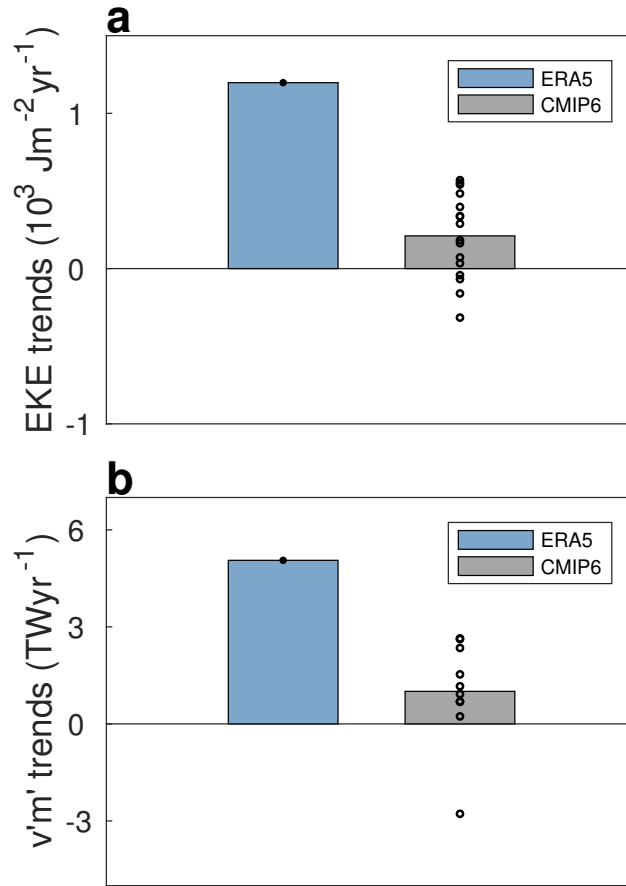

**Fig. S15.** The 1979-2018 trends in **a**, eddy kinetic energy and **b**, poleward eddy moist static energy flux in ERA5 (blue) and CMIP6 mean (gray). The black circles show the trends from the individual models/ERA5, where filled (open) circles show trends that are (not) statistically significant at the 95% level based on a Student's t-test.
